# Supplementary material for: Pairwise Distance Distillation for Unsupervised Real-World Image Super-Resolution
Source: arXiv:2407.07302 source file (2024-07-10)
Supplement: Supplementary file 1 [file fig11.tex]

\begin{figure}[!h]
    \centering
    \InsertSubfig{0.15}{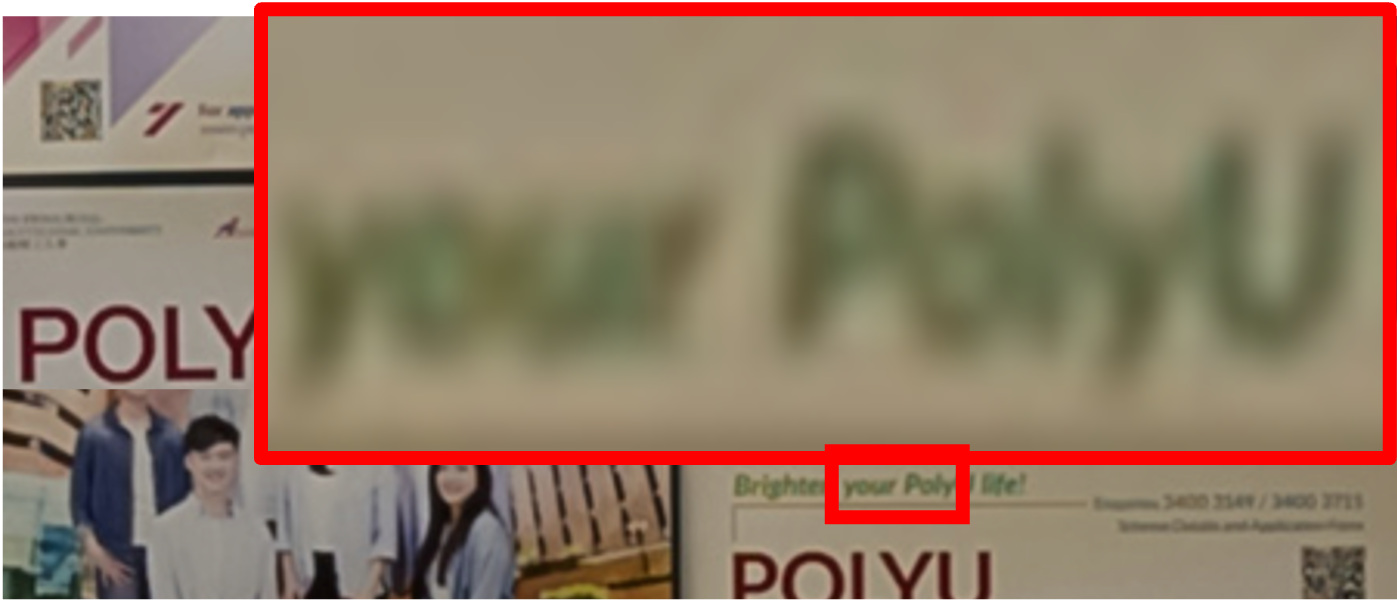}
    \InsertSubfig{0.15}{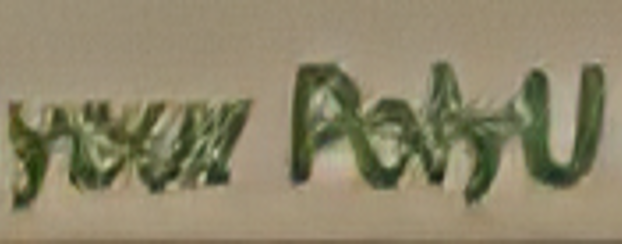}
    \InsertSubfig{0.15}{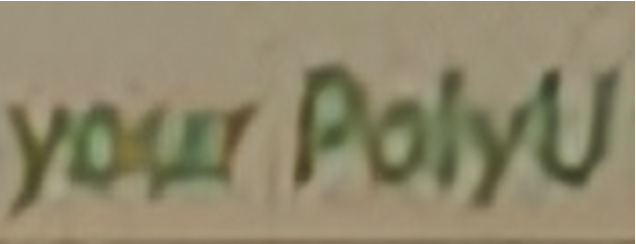}
    \InsertSubfig{0.15}{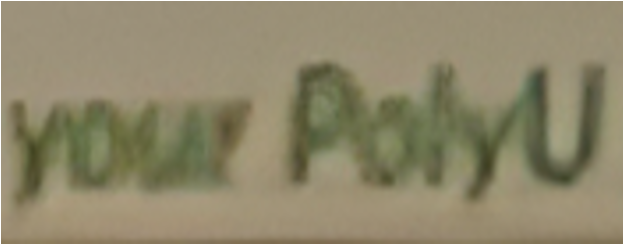}
    \InsertSubfig{0.15}{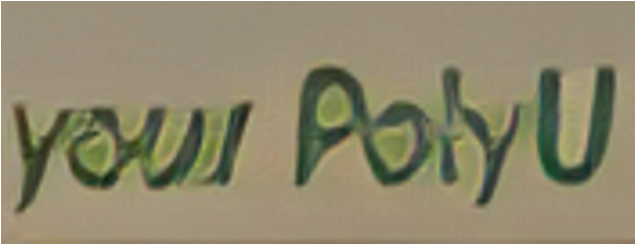}
    \InsertSubfig{0.15}{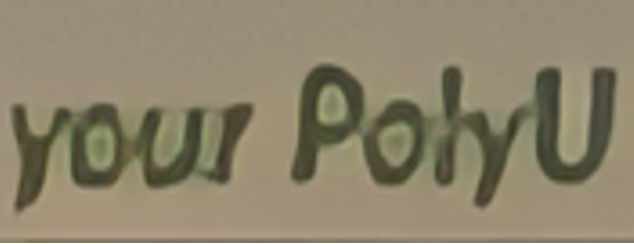}
    
    % \InsertSubfig{0.15}{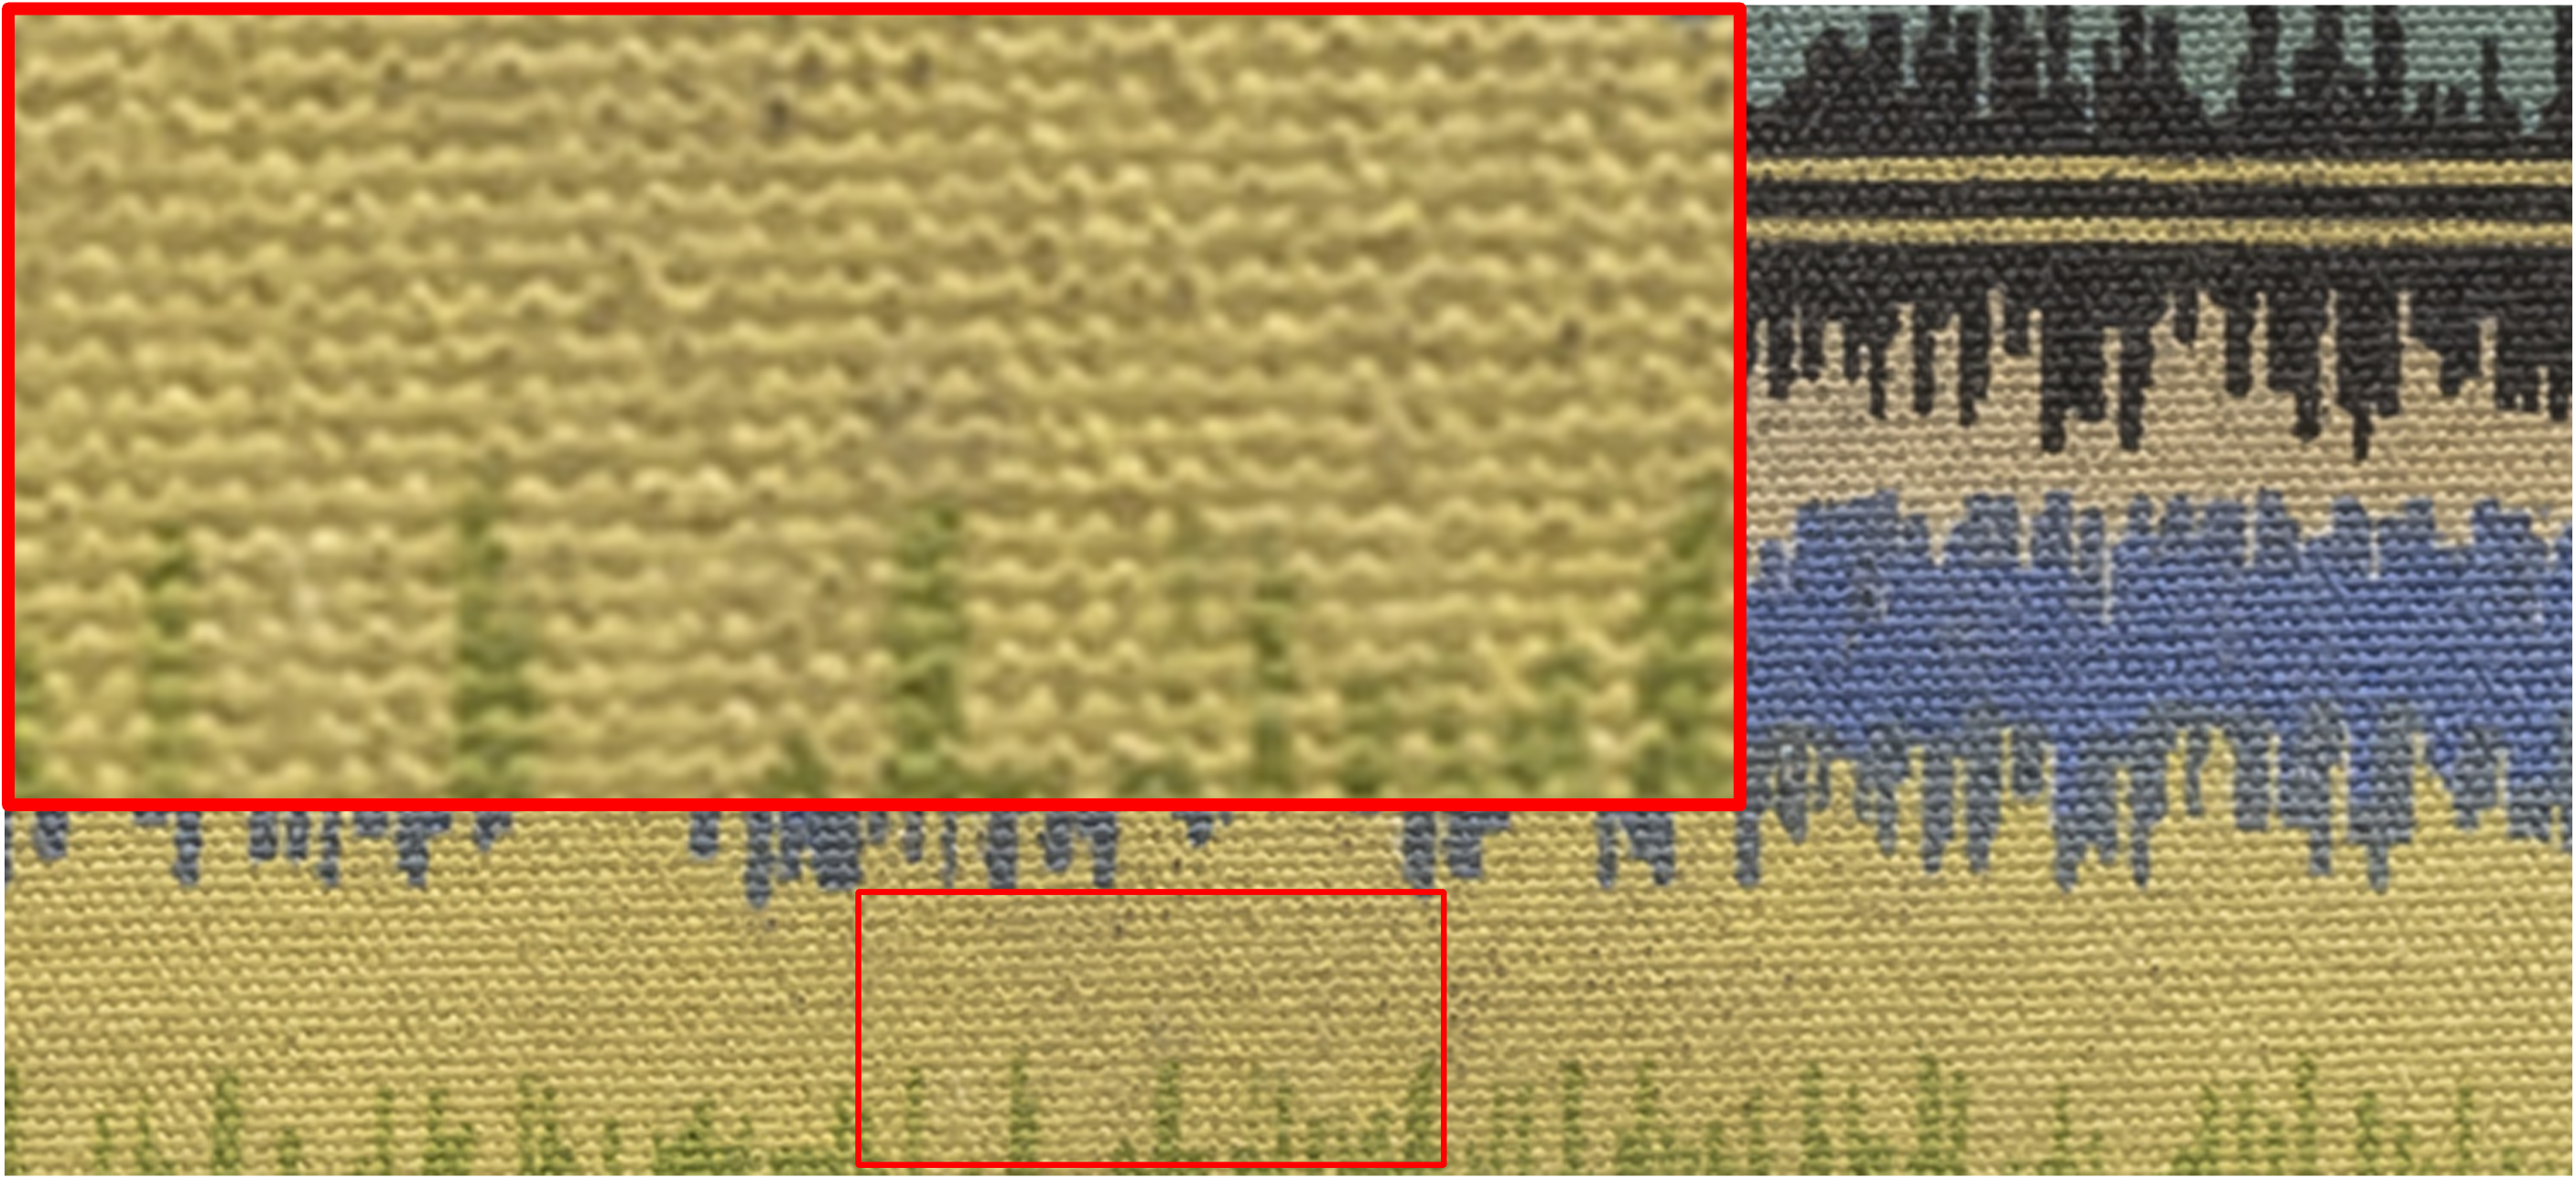}
    % \InsertSubfig{0.15}{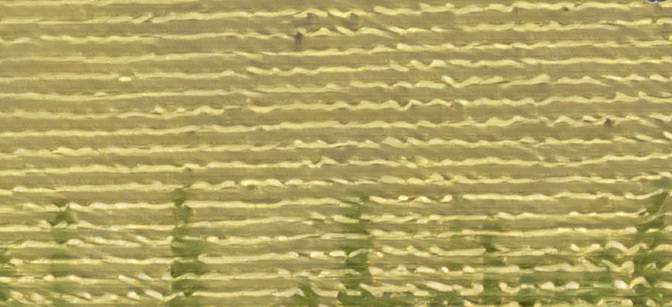}
    % \InsertSubfig{0.15}{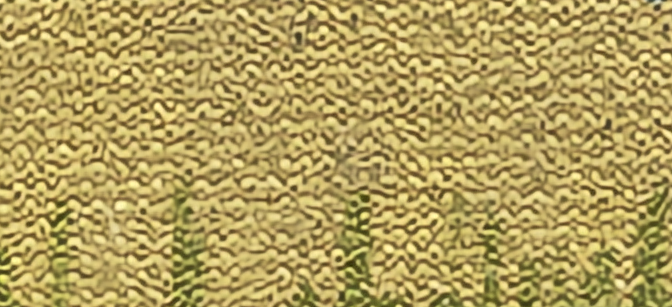}
    % \InsertSubfig{0.15}{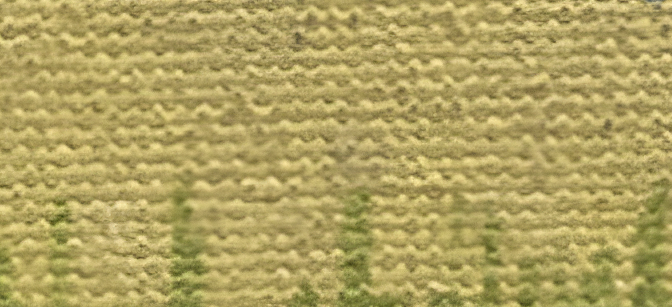}
    % \InsertSubfig{0.15}{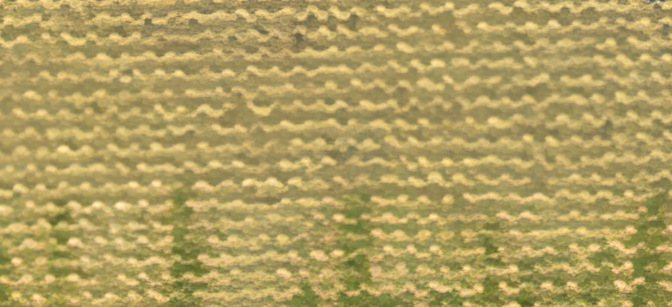}
    % \InsertSubfig{0.15}{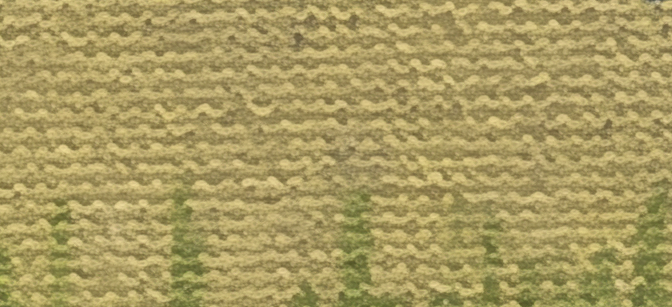}
    
    \InsertSubfig{0.15}{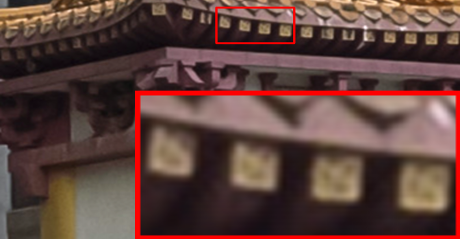}
    \InsertSubfig{0.15}{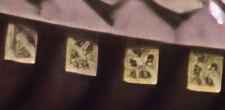}
    \InsertSubfig{0.15}{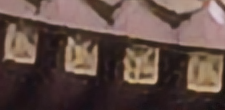}
    \InsertSubfig{0.15}{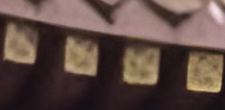}
    \InsertSubfig{0.15}{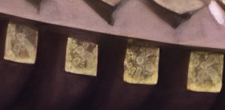}
    \InsertSubfig{0.15}{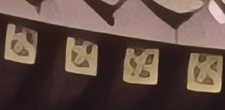}
    
    \InsertSubfig{0.15}{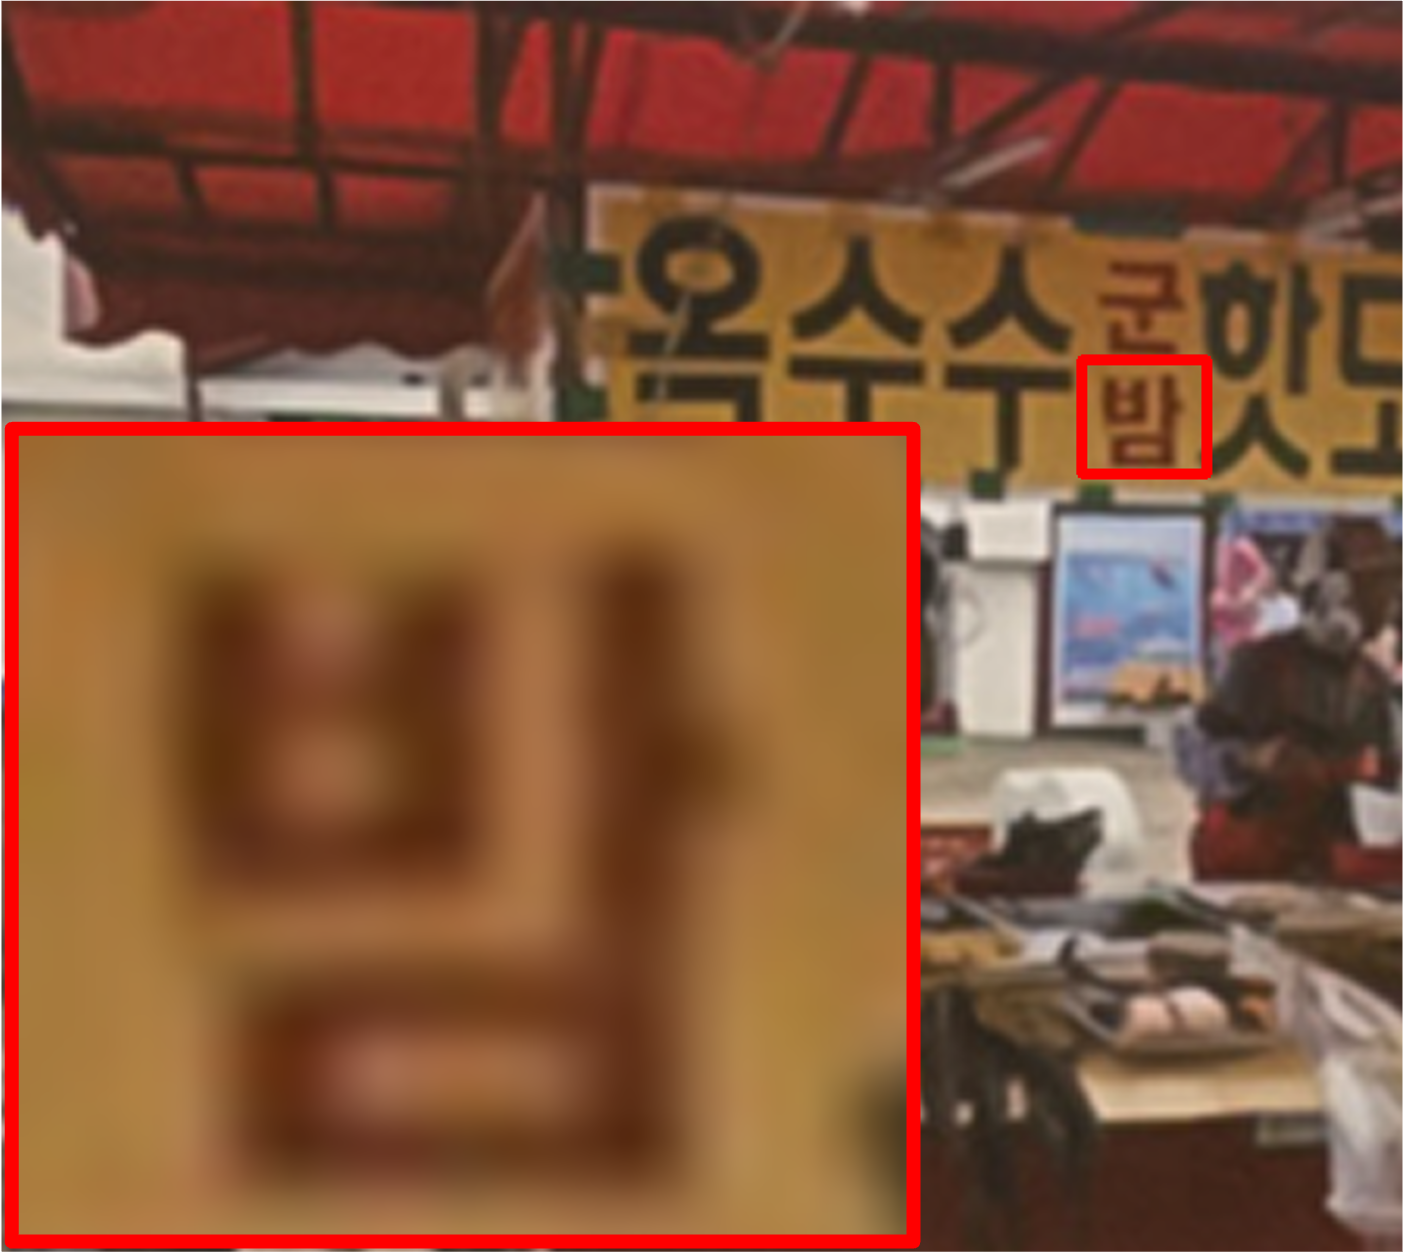}
    \InsertSubfig{0.15}{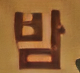}
    \InsertSubfig{0.15}{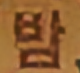}
    \InsertSubfig{0.15}{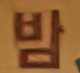}
    \InsertSubfig{0.15}{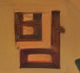}
    \InsertSubfig{0.15}{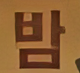}
    
    \InsertSubfig{0.15}{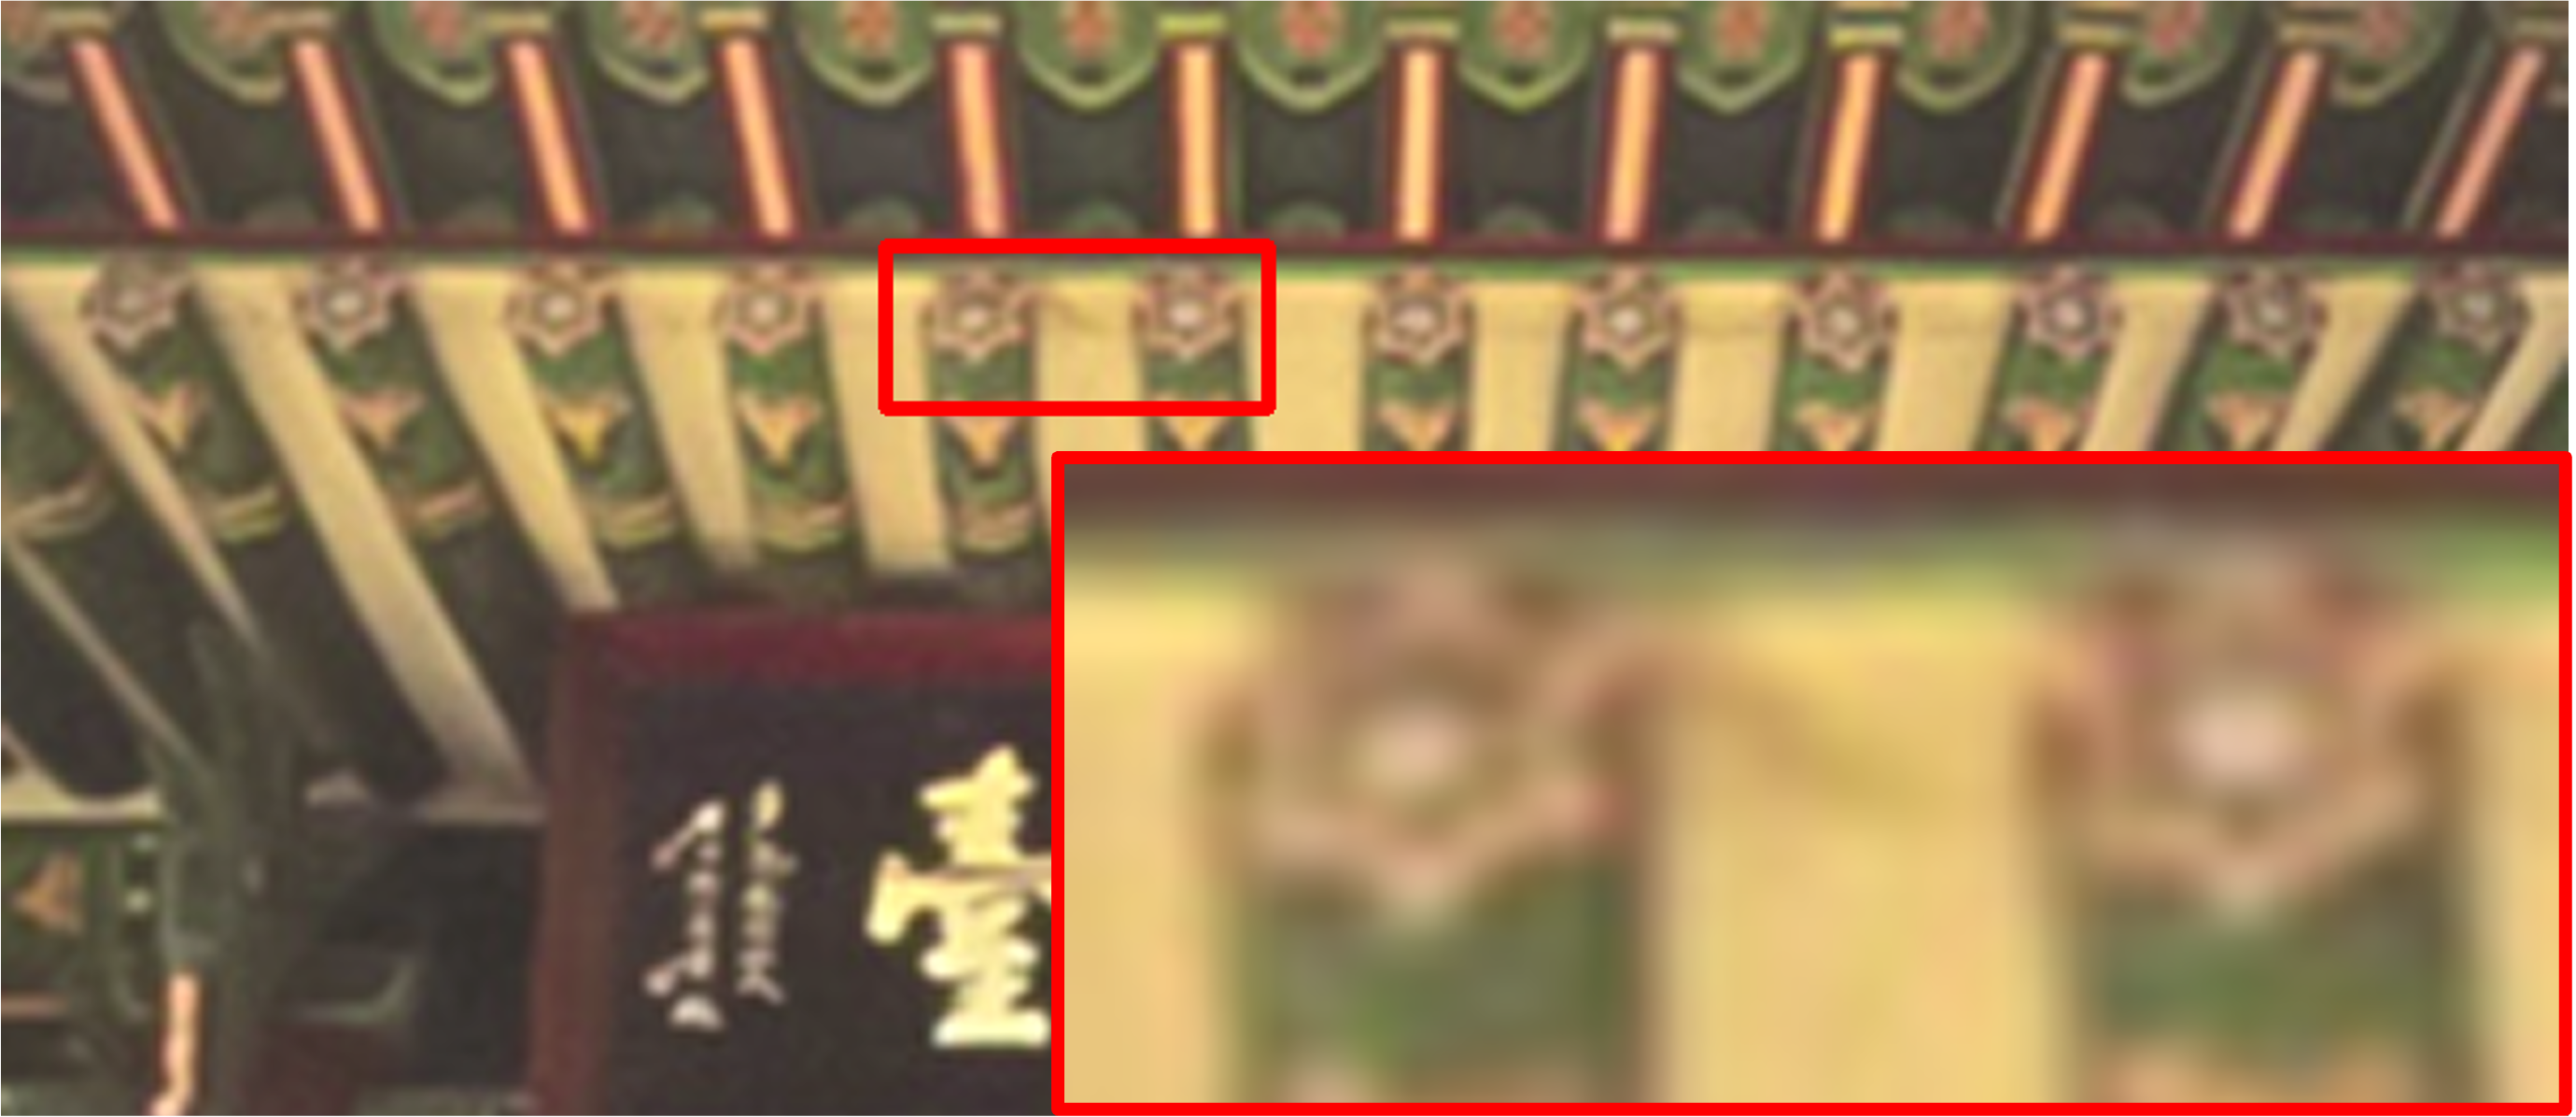}
    \InsertSubfig{0.15}{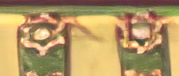}
    \InsertSubfig{0.15}{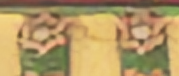}
    \InsertSubfig{0.15}{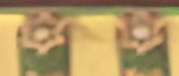}
    \InsertSubfig{0.15}{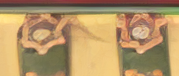}
    \InsertSubfig{0.15}{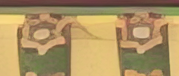}
    
    \InsertSubfig{0.15}{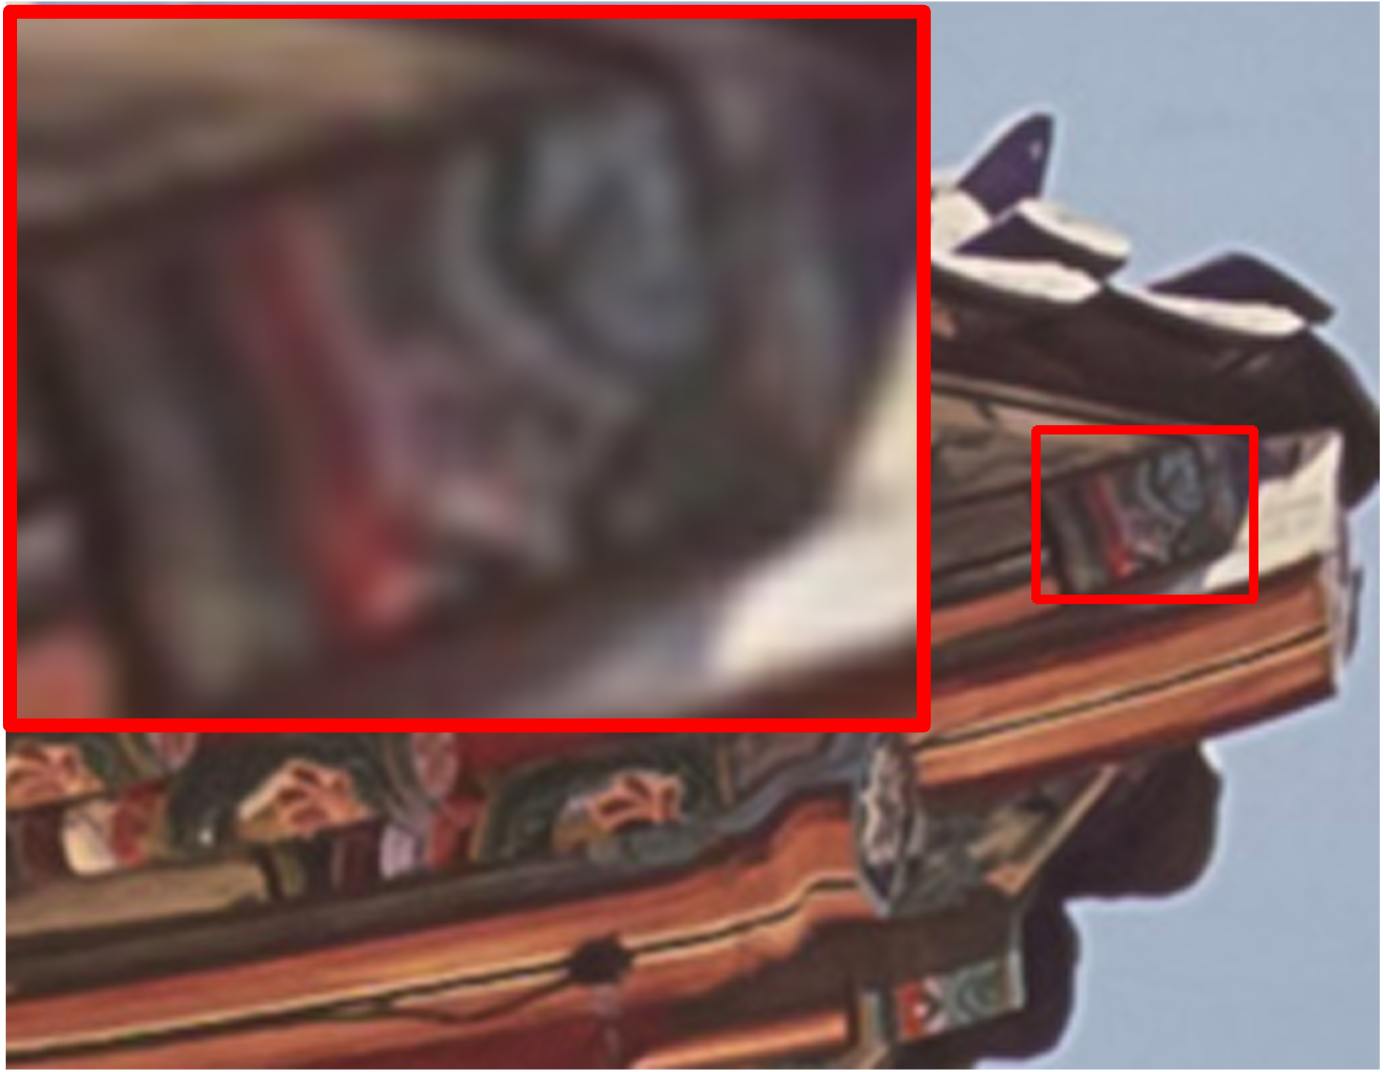}
    \InsertSubfig{0.15}{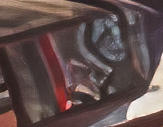}
    \InsertSubfig{0.15}{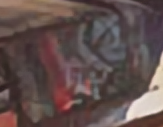}
    \InsertSubfig{0.15}{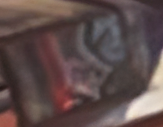}
    \InsertSubfig{0.15}{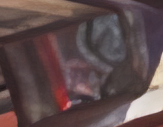}
    \InsertSubfig{0.15}{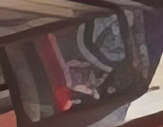}

    \InsertSubfig{0.15}{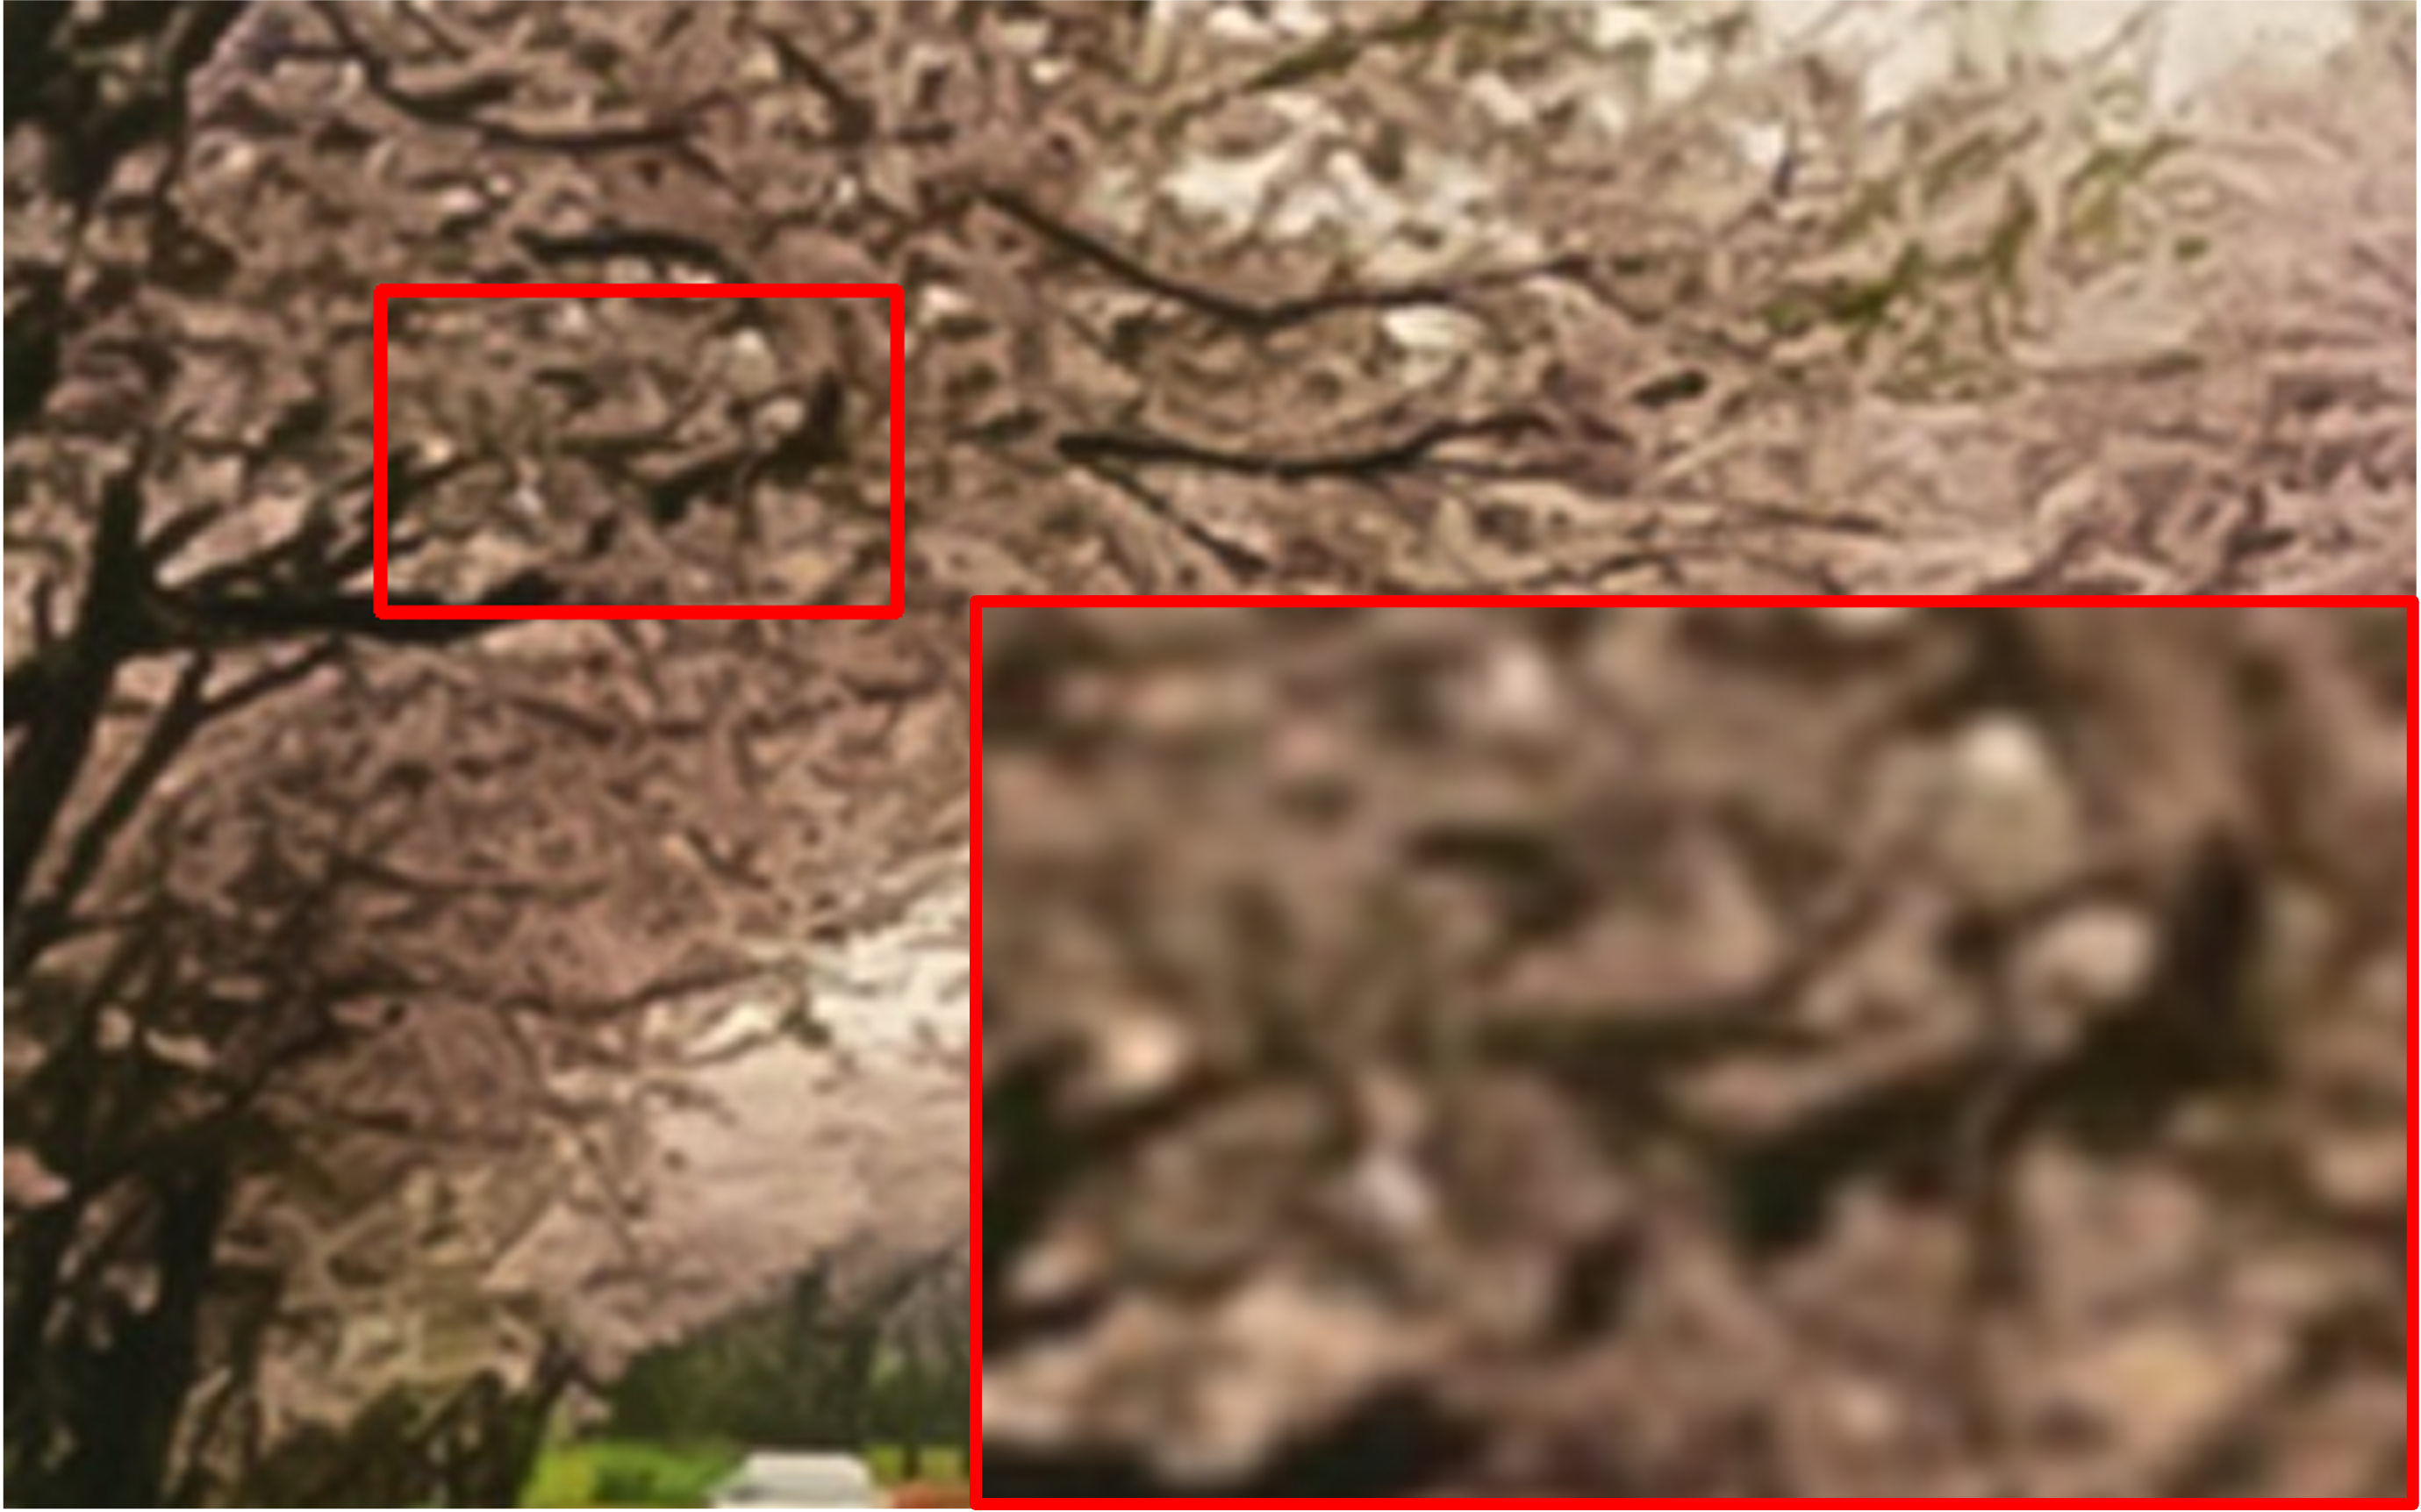}
    \InsertSubfig{0.15}{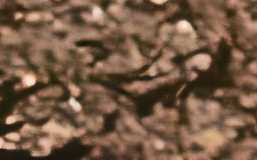}
    \InsertSubfig{0.15}{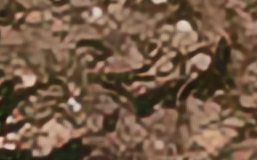}
    \InsertSubfig{0.15}{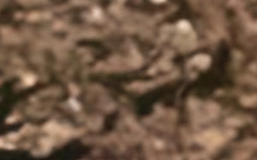}
    \InsertSubfig{0.15}{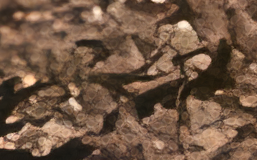}
    \InsertSubfig{0.15}{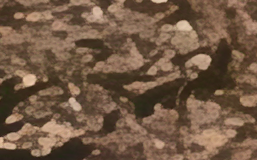}

    \InsertSubfigWithCap{0.15}{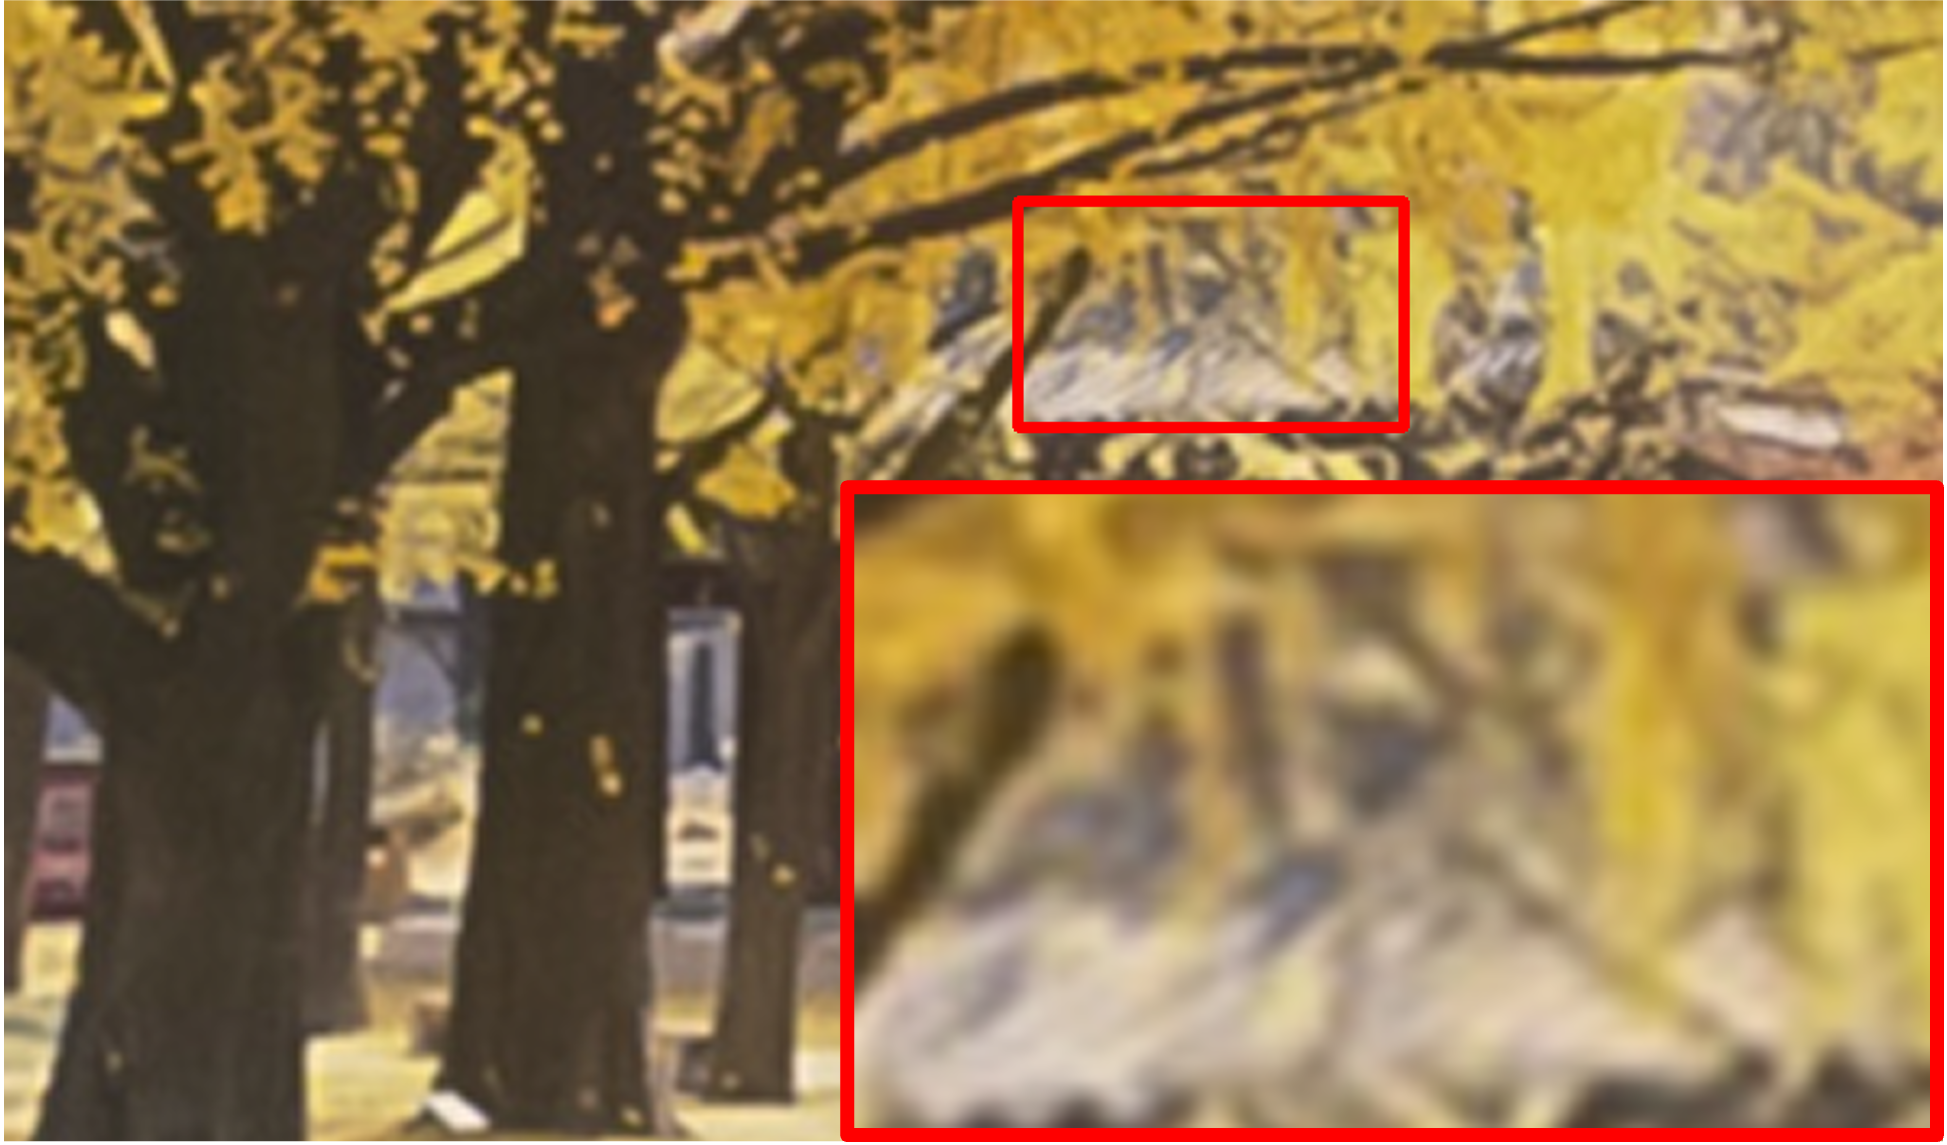}{LR}
    \InsertSubfigWithCap{0.15}{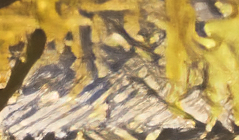}{FeMaSR}
    \InsertSubfigWithCap{0.15}{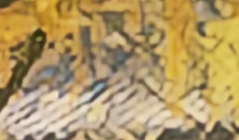}{DASR}
    \InsertSubfigWithCap{0.15}{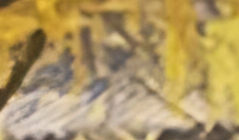}{EDAN}
    \InsertSubfigWithCap{0.15}{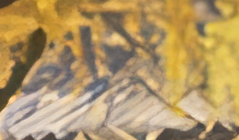}{BSRGAN}
    \InsertSubfigWithCap{0.15}{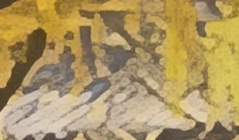}{BG+Ours}
    
    \caption{Visual comparisons with state-of-the-art methods. }
    \label{fig:suppl_visual_sota}
\end{figure}
