# Supplementary material for: Pairwise Distance Distillation for Unsupervised Real-World Image Super-Resolution
Source: arXiv:2407.07302 source file (2024-07-10)
Supplement: Supplementary file 2 [file fig12.tex]

% \begin{figure}[!h]
%     \centering
%     \InsertSubfig{0.235}{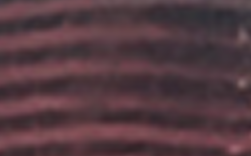}
%     \InsertSubfig{0.235}{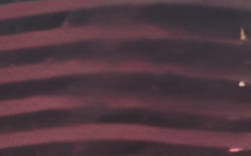}
%     \InsertSubfig{0.235}{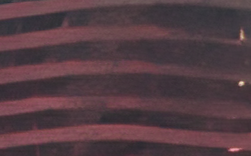}
%     \InsertSubfig{0.235}{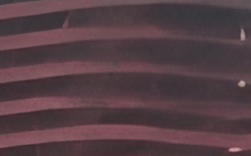}
%     % \InsertSubfig{0.235}{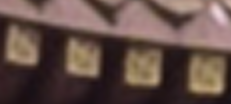}
%     % \InsertSubfig{0.235}{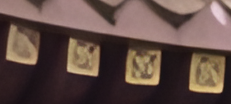}
%     % \InsertSubfig{0.235}{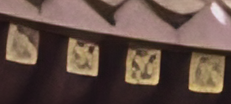}
%     % \InsertSubfig{0.235}{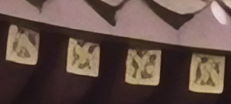}

%     \InsertSubfig{0.235}{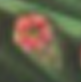}
%     \InsertSubfig{0.235}{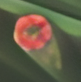}
%     \InsertSubfig{0.235}{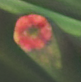}
%     \InsertSubfig{0.235}{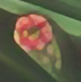}

%     \InsertSubfigWithCap{0.235}{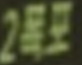}{Zoomed LR}
%     \InsertSubfigWithCap{0.235}{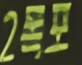}{ND}
%     \InsertSubfigWithCap{0.235}{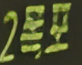}{Static}
%     \InsertSubfigWithCap{0.235}{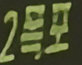}{EMA}
%     \caption{Visual comparison between Naive Distillation (ND), static version, and EMA version of our method. \YZ{change the third row}}
%     \label{fig:suppl_visual_ema}
% \end{figure}

\begin{figure}[!h]
    \centering
    \begin{minipage}{0.35\linewidth}
    \InsertSubfigWithCap{0.4}{Figures/Experiments/pddm_alt/LR_Canon_049.png}{LR}
    \InsertSubfigWithCap{0.4}{Figures/Experiments/pddm_alt/HF_ND.png}{ND}
    
    \InsertSubfigWithCap{0.4}{Figures/Experiments/pddm_alt/HF_static.png}{Static}
    \InsertSubfigWithCap{0.4}{Figures/Experiments/pddm_alt/HF_EMA.png}{EMA}
    \end{minipage}
    \begin{minipage}{0.4\linewidth}
    \InsertSubfigWithCap{1}{Figures/Experiments/pddm_alt/Mix.png}{RPS}
    \end{minipage}
    \caption{{(b-d) visualize high-frequency (HF) components of predictions for (a). Compared to ND, our methods reconstruct more HF information, and the EMA version achieves the best. (e) Radial Power Spectrum (RPS) of predictions. A larger Radial Distance refers to a higher frequency. ND has lower power in the HF region with a larger radial distance.}}
    \label{fig:suppl_visual_ema}
\end{figure}
