# Supplementary material for: Pairwise Distance Distillation for Unsupervised Real-World Image Super-Resolution
Source: arXiv:2407.07302 source file (2024-07-10)
Supplement: Supplementary file 3 [file fig9.tex]

\begin{figure}
    \centering
    \InsertSubfig{0.15}{Figures/Suppl/Fig9/LR_canon_005.png}
    \InsertSubfig{0.15}{Figures/Suppl/Fig9/aponly_canon_005.png}
    \InsertSubfig{0.15}{Figures/Suppl/Fig9/ctonly_canon_005.png}
    \InsertSubfig{0.15}{Figures/Suppl/Fig9/ours_canon_005.png}

    \InsertSubfig{0.15}{Figures/Suppl/Fig9/LR_canon_017.png}
    \InsertSubfig{0.15}{Figures/Suppl/Fig9/aponly_canon_017.png}
    \InsertSubfig{0.15}{Figures/Suppl/Fig9/ctonly_canon_017.png}
    \InsertSubfig{0.15}{Figures/Suppl/Fig9/ours_canon_017.png}

    \InsertSubfigWithCap{0.15}{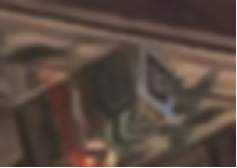}{LR}
    \InsertSubfigWithCap{0.15}{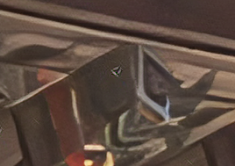}{$R_{inter}$}
    \InsertSubfigWithCap{0.15}{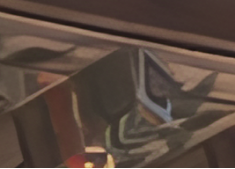}{$R_{intra}$}
    \InsertSubfigWithCap{0.15}{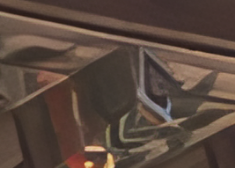}{Ours}
    \caption{Visual examples for methods in \cref{tab:suppl_static_abla_loss}. Using $R_{inter}$ only yields artifact points, while $R_{intra}$ only produce blurry patterns.}
    \label{fig:suppl_static_visual}
\end{figure}
